# Supplementary material for: Controllable Lexical Simplification for English
Source: arXiv:2302.02900 source file (2023-02-06)
Supplement: Supplementary file 1 [file appendix.tex]

\section{Qualitative Evaluation Examples} \label{appendix:qualitative_evaluation_examples}

\begin{table*}[htb]
\label{table_results_full_pipeline}
\tiny
\begin{center}

 %\begin{adjustbox}{width=\textwidth}
\begin{tabular}{|c|c|c|c|c|c|c|c|c|c|c|}
      \hline
 	 Example 1 &  \multicolumn{10}{l|}{"It originally {\bf aired} on the Fox network in the United States on October 10 , 1991 ."}	
   \\
 	 \cline{2-11}
	GOLD &\multicolumn{10}{l|}{  \underline{showed} (16), played (12) ,shown (4),appeared (2),televised,ran,premiered,opened,broadcasted, }\\
	\hline
	\hline
    LSBert & \\
    \hline
    ConLS &  \cellcolor{orange!50}aired &\cellcolor{cyan!25}	broadcast	& \cellcolor{orange!50}airs	& \cellcolor{green!25}showed & \cellcolor{yellow!25}	seen &\cellcolor{green!25}	ran	& \cellcolor{red!25}lived	& \cellcolor{red!25}came	& \cellcolor{red!25}began	& \cellcolor{magenta!25} radiated  \\
    \hline
\hline

      \hline
 	 Example 2 & \multicolumn{10}{l|}{A good measure of notability is whether someone has been featured in {\bf multiple} , independent , reliable sources . } \\
 	\cline{2-11}
	GOLD & \multicolumn{10}{l|}{    \underline{many} (29), several (11), different (5), numerous, trotting, some} \\
	\hline
	\hline
    LSBert & \\
    \hline
    ConLS & 	\cellcolor{green!25}many	& \cellcolor{orange!50} multiple &\cellcolor{green!25}	numerous &\cellcolor{green!25}	several &  \cellcolor{red!25}	number &  \cellcolor{red!25}	a number	&  \cellcolor{red!25} more	 &  \cellcolor{red!50} few	&  \cellcolor{yellow!25} various	&  \cellcolor{red!25} numbers\\
    \hline
\hline

      \hline
 	 Example 3 &  \multicolumn{10}{l|}{he normally appears in a running gag, where he usually suffers {\bf unfortunate}, nearly always fatal, events.}   \\
 	\cline{2-11}
GOLD & \multicolumn{10}{l|}{    \underline{bad} (19), unlucky (15), sad (6), terrible (3), unhappy(2), hapless, tragic, unlikely, damaging, disasterous}\\

	\hline
	\hline
    LSBert & \\
    \hline
    ConLS &\cellcolor{green!25}bad	& \cellcolor{green!25}unlucky	& 	\cellcolor{red!25}wrong	& 	\cellcolor{red!25}frustrating		& \cellcolor{yellow!25}disastrous	& \cellcolor{red!25}unexpected	& \cellcolor{red!25}unusual		& \cellcolor{red!25}difficult	& 	\cellcolor{red!25}unfortunately		&\cellcolor{red!25} troubling \\
    \hline
\hline

      \hline
 	 Example 4 & \multicolumn{10}{l|}{ Tolstoy was born in Yasnaya Polyana, the family {\bf estate} in the Tula region of Russia.}   \\
 	\cline{2-11}
	GOLD & \multicolumn{10}{l|}{  \underline{home}(31), property (5), house (4), residence (3), lands(2), land(2), domain, grounds}\\
	\hline
	\hline
    LSBert & \\
    \hline
    ConLS & \cellcolor{green!25}house &	\cellcolor{green!25}home  &	\cellcolor{orange!50}estate  &	\cellcolor{yellow!25} place &	\cellcolor{green!25}	residence  &	\cellcolor{yellow!25}	site	 &\cellcolor{red!25}	hold &	\cellcolor{red!25}	country	 &	\cellcolor{yellow!25}stead  &	\cellcolor{yellow!25}	building\\
    \hline
\hline

      \hline
 	 Example 5 &  \multicolumn{10}{l|}{Gygax is {\bf generally} acknowledged as the father of role-playing games.}
  \\
 	 \cline{2-11}
	GOLD & \multicolumn{10}{l|}{  \underline{usually} (28), normally (5), mainly (5), often (3), mostly (2), widely (2), commonly (2), traditionally, roughly}\\
	\hline
	\hline
    LSBert & \\
    \hline
    ConLS & \cellcolor{green!25} usually &   \cellcolor{green!25} mostly &  \cellcolor{green!25}  	widely &  \cellcolor{yellow!25} 	largely &   \cellcolor{yellow!25}	in general &  \cellcolor{yellow!25} 	typically &	\cellcolor{green!25}normally &  \cellcolor{green!25} 	often &  \cellcolor{red!25} 	well\\
    \hline
\hline

      \hline
 	 Example 6 & \multicolumn{10}{l|}{he is notable as a {\bf performer} of Australian traditional folk songs in an authentic style.}
 
  \\
 	 \cline{2-11}
	GOLD & \multicolumn{10}{l|}{ \underline{singer} (27), entertainer (6), musician (5), artist (5), player(4), actor(2), worker}\\
	\hline
	\hline
    LSBert & \\
    \hline
    ConLS & \cellcolor{orange!50}performer &   \cellcolor{green!25}	singer &  \cellcolor{green!25}  	player &   \cellcolor{green!25} 	interpreter &  \cellcolor{red!25} writer &  \cellcolor{red!25}recorder &    \cellcolor{red!25}	composer &   \cellcolor{red!25}	producer &   \cellcolor{red!25}	conductor &   \cellcolor{yellow!25}	musician \\
    \hline
\hline

      \hline
 	 Example 7 & \multicolumn{10}{l|}{Aung San Suu Kyi returned to Burma in 1988 to take care of her {\bf ailing} mother.}
  \\
 	 \cline{2-11}
	GOLD & \multicolumn{10}{l|}{ \underline{sick} (36), ill (5), sickly (3), dying (3), suffering (2), distressed, sickening}\\

	\hline
	\hline
    LSBert & \\
    \hline
    ConLS &   \cellcolor{green!25}   ill &    \cellcolor{green!25}  	dying &   \cellcolor{red!25}   	dead &    \cellcolor{green!25}  	sick &    \cellcolor{magenta!25}  	infirm &   \cellcolor{red!25}   	deteriorating &   	 \cellcolor{orange!50}   ailing &   \cellcolor{red!25}   	failing &    \cellcolor{yellow!25}  	unwell &   \cellcolor{red!25}   	wounded \\
    \hline
\hline

      \hline
 	 Example 8 & \multicolumn{10}{l|}{the Convent has been the official {\bf residence} of the Governor of Gibraltar since 1728.}

  \\
 	 \cline{2-11}
	GOLD & \multicolumn{10}{l|}{ \underline{home} (40), house (6), dwelling (2), abode, owner, people}\\

	\hline
	\hline
    LSBert & \\
    \hline
    ConLS & \cellcolor{green!25} home &  \cellcolor{green!25} 	house &   \cellcolor{yellow!25}	place &   \cellcolor{red!25}	office &  \cellcolor{green!25} 	base &  \cellcolor{red!25} 	room &   	\cellcolor{yellow!25} quarters & \cellcolor{red!25}  	resident &   \cellcolor{green!25}	abode &   \cellcolor{yellow!25}	stay \\
    \hline
\hline

      \hline
 	 Example 9 &  \multicolumn{10}{l|}{Kowal suggested the name and the IAU {\bf endorsed} it in 1975.}

  \\
 	 \cline{2-11}
	GOLD & \multicolumn{10}{l|}{  \underline{supported} (21), approved (15), accepted (4), backed (2), okayed (2), authorized (2), favored, passed, adopted, ratified}\\
\hline
	\hline
    LSBert & \\
    \hline
    ConLS  & \cellcolor{green!25} approved &   \cellcolor{orange!50}	endorsed &  \cellcolor{green!25} 	accepted &  \cellcolor{green!25} 	adopted &   \cellcolor{green!25}	supported &  \cellcolor{yellow!25} 	loved &   \cellcolor{yellow!25}	recommended &   \cellcolor{yellow!25}	backed &  \cellcolor{red!25} 	approve &   \cellcolor{red!25}	affirmed \\
    \hline
\hline

      \hline
 	 Example 10 &  \multicolumn{10}{l|}{it overwinters in  {\bf conifer} groves .}
  \\
 	 \cline{2-11}
	GOLD & \multicolumn{10}{l|}{  \underline{tree} (16),  \underline{pine} (16), evergreen (2), fir, wood, cedar, grassy, nice}\\
	\hline
	\hline
    LSBert & \\
    \hline
    ConLS &  \cellcolor{orange!50} conifer & \cellcolor{red!25}  spruce &   \cellcolor{green!25}	pine &   \cellcolor{green!25}	tree &   \cellcolor{green!25}	fir &  \cellcolor{red!25} 	prune &  \cellcolor{green!25} 	wood &  \cellcolor{red!25} 	forest &  \cellcolor{red!25} 	reed &   \cellcolor{red!25}	beech \\
    \hline
\hline

\end{tabular}
\label{qualitative_evaluation}
  %\end{adjustbox}
	\caption{{\small Comparison of top-10 results of the LSBert ant CoLS approaches on the LexMTurk dataset. Note: we assume that there are some few errors in gold-annotations in LexMturk. 
    \\
     Colour legend:\\
     \hline
     \vspace{0.25cm}
    \textcolor{green!25}{$\blacksquare$} = correct substitution reported by the annotators\\
    \textcolor{yellow!25}{$\blacksquare$} = correct substitution not reported by the annotators\\ 
    \textcolor{cyan!25}{$\blacksquare$} = correct substitution reported by the annotators but without correct morphological inflection\\ \textcolor{orange!50}{$\blacksquare$} = the same target complex word (or a morphological variation of it)\\
    \textcolor{magenta!25}{$\blacksquare$} = valid substitution but incorrect simplification (substitution more complex than the original target word)\\
    \textcolor{red!25}{$\blacksquare$} = incorrect substitution\\
    \textcolor{red!50}{$\blacksquare$} = antonym\\
    
        \hline 
}

 }
\end{center}
\end{table*}
